# Supplementary material for: Ternary oxides of $\textit{s}$- and $\textit{p}$-block metals for photocatalytic solar-to-hydrogen conversion
Source: arXiv:2303.03332 source file (2023-12-18)
Supplement: Supplementary file 1 [file supplemental_material.pdf]

# Supplemental Material for "Ternary oxides of *s*- and *p*-block metals for photocatalytic solar-to-hydrogen conversion"

Simon Gelin, Nicole E. Kirchner-Hall, Rowan R. Katzbaer, Monica Theibault, Yihuang Xiong, Wayne Zhao, Mohammed M. Khan, Eric Andrewlavage, Paul Orbe, Steven Baksa, Matteo Cococcioni, Iurii Timrov, Quinn Campbell, Héctor Abruña, Raymond Schaak, and Ismaila Dabo

## CONTENTS

I. First-principles predictions from generalized-gradient calculations 1

II. Projected density of states before and after self-interaction correction 5

III. Electrochemical stability from computed Pourbaix diagrams 7

IV. Experimental data from structural and optical measurements 12

References 13

## I. FIRST-PRINCIPLES PREDICTIONS FROM GENERALIZED-GRADIENT CALCULATIONS

The candidate photocatalysts studied here are ternary oxide compounds made of *s*-block metal cations (Li, Na, K, Rb, Cs, Mg, Ca, Sr, Ba) and closed-shell ($d^{10}$) *p*-block metal cations (In, Sn, Sb, Pb, Bi). The list of candidate materials was extracted from the *Materials Project* database. After a first screening based on toxicity, radioactivity, and abundance (cf. main text), the list was reduced to 109 materials. The chemical formula of these materials, the space group they belong to, and their band gap and band edges evaluated within generalized-gradient DFT are reported in Table S1. The 14 materials that have a unit cell with more than 50 atoms and were thus not included in the study are: $Na_5InO_4$, $K_{14}In_4O_{13}$, $K_5InO_4$, $K_4SnO_3$, $Rb_2Sb_8O_{13}$, $Rb_3Sb_5O_{14}$, $Cs_3Sb_5O_{14}$, $Sr_5(Sb_{11}O_{19})_2$, $K_4PbO_3$, $Rb_4PbO_3$, $KBiO_3$, $Rb_2Bi_4O_7$, $Cs_2Bi_4O_7$, $Ca(BiO_2)_2$.

TABLE S1: Predicted band gaps and band edges using the PBEsol exchange-correlation functional for 109 ternary oxides of *s*- and *p*-block metal elements, grouped by indates, stannates, antimonates, plumbates, and bismuthates. Less than 10% of the material calculations failed due to convergence issues, and these materials are indicated throughout the table.

| **Chemical formula** | **Space group** | **DFT predictions** (eV) $\varepsilon_g$ | $E_{VB}$ | $E_{CB}$ |
|---|---|---|---|---|
| $LiInO_2$ | $I4_1/amd$ | 1.96 | 1.34 | –0.62 |
| $Li_3InO_3$ | $P\bar{3}1c$ | 3.08 | 1.58 | –1.50 |
| $NaInO_2$ | $R\bar{3}m$ | 2.02 | 1.30 | –0.72 |
| $Na_5InO_4$ | $Pmmn$ | 1.82 | 0.71 | –1.11 |
| $Cs_3InO_3$ | $P2_1/c$ | 2.30 | 0.61 | –1.69 |
| $Cs_8In_2O_7$ | $P2_1/c$ | 2.06 | 0.38 | –1.68 |
| $CsIn_3O_5$ | $Pnma$ | 1.59 | 1.24 | –0.35 |
| $SrIn_2O_4$ | $Pnma$ | 1.96 | 1.38 | –0.58 |
| $Sr_2In_2O_5$ | $Ima2$ | 1.02 | 0.68 | –0.34 |
| $Ba_3In_2O_6$ | $I4/mmm$ | 1.03 | 0.77 | –0.26 |
| $Ba_2In_2O_5$ | $Ima2$ | — | — | — |
| $Ba_4In_6O_{13}$ | $Iba2$ | — | — | — |

Continued on next page

TABLE S1 – continued from previous page

| **Chemical formula** | **Space group** | **DFT predictions** (eV) | | |
|---|---|---|---|---|
| | | $\varepsilon_g$ | $E_{VB}$ | $E_{CB}$ |
| $Li_8SnO_6$ | $R\bar{3}$ | 4.09 | 2.06 | –2.04 |
| $Li_2SnO_3$ | $C2/c$ | 3.32 | 2.27 | –1.04 |
| $Na_4SnO_4$ | $P\bar{1}$ | 2.16 | 1.24 | –0.92 |
| $Na_4SnO_3$ | $Cc$ | 1.90 | 0.83 | –1.07 |
| $K_2Sn_2O_3$ | $I2_13$ | 1.35 | 0.88 | –0.47 |
| $K_2SnO_3$ | $Pnma$ | 2.30 | 1.41 | –0.89 |
| $K_4SnO_4$ | $P\bar{1}$ | 2.48 | 1.08 | –1.41 |
| $Rb_4SnO_4$ | $P\bar{1}$ | 2.30 | 0.92 | –1.38 |
| $Rb_2SnO_2$ | $P2_12_12_1$ | 2.24 | 0.90 | –1.34 |
| $Rb_2Sn_2O_3$ | $R\bar{3}m$ | 0.94 | 0.62 | –0.31 |
| $Cs_4SnO_4$ | $P2_1/c$ | 2.59 | 0.93 | –1.65 |
| $Cs_2Sn_2O_3$ | $Pnma$ | 2.54 | 1.34 | –1.20 |
| $Ca_2SnO_4$ | $Pbam$ | 2.87 | 1.89 | –0.98 |
| $CaSnO_3$ | $R\bar{3}$ | 3.09 | 2.37 | –0.72 |
| $SrSnO_3$ | $Pnma$ | 2.04 | 1.75 | –0.29 |
| $Sr_2SnO_4$ | $P4_2/ncm$ | 2.92 | 1.78 | –1.14 |
| $Sr_3Sn_2O_7$ | $Cmcm$ | 2.46 | 1.72 | –0.74 |
| $BaSnO_3$ | $Pm\bar{3}m$ | 0.85 | 1.34 | 0.50 |
| $Ba_2SnO_4$ | $I4/mmm$ | 2.78 | 1.97 | –0.81 |
| $Li_3SbO_4$ | $P2/c$ | 3.24 | 2.23 | –1.00 |
| $Li_5SbO_5$ | $C2/m$ | 3.08 | 1.87 | –1.21 |
| $LiSbO_3$ | $Pnna$ | 2.31 | 2.46 | 0.15 |
| $LiSb_3O_8$ | $P2_1/c$ | 1.14 | 2.38 | 1.25 |
| $Li_7SbO_6$ | $R3$ | 3.70 | 2.03 | –1.68 |
| $LiSbO_2$ | $P2_1/c$ | 2.68 | 2.27 | –0.41 |
| $NaSbO_3$ | $R\bar{3}$ | 2.79 | 2.64 | –0.15 |
| $Na_3SbO_4$ | $P2/c$ | 2.28 | 1.66 | –0.63 |
| $Na_3SbO_3$ | $I\bar{4}3m$ | 3.04 | 1.74 | –1.29 |
| $Na_2Sb_4O_7$ | $C2/c$ | 2.93 | 2.69 | –0.24 |
| $NaSb_5O_8$ | $P\bar{1}$ | 2.93 | 2.69 | –0.24 |
| $KSbO_3$ | $R3$ | 2.83 | 2.47 | –0.35 |
| $K_3SbO_4$ | $P2/c$ | 2.03 | 1.23 | –0.79 |
| $K_2Sb_4O_{11}$ | $C2/m$ | 2.02 | 2.51 | 0.50 |
| $KSb_3O_5$ | $P2_1/c$ | 2.91 | 2.75 | –0.16 |
| $K_3SbO_3$ | $P2_1/3$ | 3.32 | 1.57 | –1.75 |
| $KSbO_2$ | $C2/c$ | 1.98 | 1.63 | –0.35 |
| $Rb_2Sb_4O_{11}$ | $C2/m$ | 2.00 | 2.48 | 0.48 |
| $RbSbO_2$ | $C2/c$ | 2.22 | 1.71 | –0.51 |
| $Cs_3SbO_4$ | $Pnma$ | 2.92 | 1.50 | –1.42 |
| $Cs_4Sb_2O_5$ | $Cm$ | 2.82 | 1.40 | –1.42 |
| $Cs_3SbO_3$ | $P2_13$ | 3.28 | 1.36 | –1.92 |
| $CsSbO_2$ | $C2/c$ | 2.41 | 1.72 | –0.69 |
| $Mg(SbO_3)_2$ | $P4_2/mnm$ | 1.22 | 2.49 | 1.28 |
| $Mg(SbO_2)_2$ | $P4_2/mbc$ | 2.38 | 2.76 | 0.39 |
| $Ca_2Sb_2O_7$ | $Imma$ | 1.94 | 2.09 | 0.15 |
| $Ca(SbO_3)_2$ | $P\bar{3}m1$ | 2.82 | 2.93 | 0.11 |

Continued on next page

TABLE S1 – continued from previous page

| **Chemical formula** | **Space group** | **DFT predictions** (eV) $\varepsilon_g$ | $E_{VB}$ | $E_{CB}$ |
|---|---|---|---|---|
| $Sr(SbO_3)_2$ | $P\bar{3}m1$ | 2.91 | 2.91 | 0.00 |
| $Sr_2Sb_2O_7$ | $Imma$ | 1.56 | 1.81 | 0.25 |
| $Ba(SbO_3)_2$ | $P\bar{3}m1$ | 2.99 | 3.08 | 0.08 |
| $Ba_3(SbO_3)_2$ | $P\bar{1}$ | — | — | — |
| $Li_4PbO_4$ | $Cmcm$ | 1.49 | 0.96 | –0.52 |
| $Li_2PbO_3$ | $C2/c$ | 1.13 | 1.10 | –0.03 |
| $Li_8PbO_6$ | $R\bar{3}$ | 2.50 | 1.23 | –1.27 |
| $Na_4PbO_4$ | $P\bar{1}$ | 1.36 | 0.76 | –0.57 |
| $Na_6PbO_5$ | $Cmcm$ | – | – | – |
| $Na_2PbO_2$ | $Pbcn$ | 2.39 | 1.23 | –1.16 |
| $Na_6PbO_4$ | $I\bar{4}3m$ | 1.45 | 0.46 | –0.99 |
| $K_2PbO_3$ | $P6_3/mcm$ | 1.31 | 0.84 | –0.47 |
| $K_4PbO_4$ | $P\bar{1}$ | 1.82 | 0.70 | –1.12 |
| $K_6Pb_2O_5$ | $P\bar{1}$ | 2.20 | 0.69 | –1.51 |
| $K_2PbO_2$ | $P\bar{1}$ | 1.97 | 0.74 | –1.23 |
| $K_2Pb_2O_3$ | $I2_13$ | 1.80 | 0.97 | –0.82 |
| $K_4PbO_3$ | $Pbca$ | 2.39 | 0.69 | –1.70 |
| $Rb_2PbO_3$ | $Pnma$ | 1.39 | 0.83 | –0.56 |
| $Rb_2PbO_2$ | $P\bar{1}$ | 1.92 | 0.66 | –1.26 |
| $Rb_4PbO_3$ | $Pbca$ | 2.28 | 0.57 | –1.71 |
| $Cs_2PbO_3$ | $Cmc2_1$ | 1.60 | 0.82 | –0.77 |
| $Cs_4PbO_4$ | $P2_1/c$ | 1.88 | 0.54 | –1.34 |
| $Cs_2PbO_2$ | $P\bar{1}$ | 1.86 | 0.51 | –1.35 |
| $Ca_2PbO_4$ | $Pbam$ | 1.52 | 1.15 | –0.38 |
| $CaPbO_3$ | $Pnma$ | 1.01 | 1.23 | 0.22 |
| $Sr_2PbO_4$ | $Pbam$ | 1.46 | 0.99 | –0.47 |
| $SrPbO_3$ | $Pnma$ | 0.91 | 1.08 | 0.17 |
| $Ba_2PbO_4$ | $I4/mmm$ | 1.40 | 1.21 | –0.19 |
| $BaPbO_3$ | $C2/m$ | 0.25 | 0.94 | 0.69 |
| $LiBiO_3$ | $Pccn$ | 0.33 | 2.14 | 1.81 |
| $Li_5BiO_5$ | $Cm$ | 1.60 | 1.38 | –0.23 |
| $Li_3BiO_4$ | $P4_2/mnm$ | 1.31 | 1.63 | 0.32 |
| $NaBiO_3$ | $R\bar{3}$ | 1.27 | 2.54 | 1.27 |
| $Na_3BiO_4$ | $P2/c$ | 1.18 | 1.46 | 0.28 |
| $K_3BiO_4$ | $P\bar{1}$ | 1.37 | 1.24 | –0.13 |
| $Mg(BiO_3)_2$ | $P4_2/mnm$ | 0.09 | 2.76 | 2.66 |
| $Li_3BiO_3$ | $P\bar{1}$ | — | — | — |
| $LiBiO_2$ | $Ibam$ | 2.22 | 2.83 | 0.61 |
| $NaBiO_2$ | $C2/c$ | 0.96 | 2.12 | 1.16 |
| $Na_3BiO_3$ | $I\bar{4}3m$ | 2.98 | 2.10 | –0.88 |
| $KBiO_2$ | $C2/c$ | 1.66 | 2.23 | 0.56 |
| $K_3BiO_3$ | $I\bar{4}3m$ | 3.02 | 1.77 | –1.24 |
| $K_4Bi_2O_5$ | $P\bar{1}$ | 2.64 | 1.97 | –0.67 |
| $Rb_3BiO_3$ | $P2_13$ | 3.30 | 1.85 | –1.45 |
| $RbBiO_2$ | $C2/c$ | 2.17 | 2.43 | 0.26 |
| $CsBiO_2$ | $C2/c$ | 2.38 | 2.43 | 0.05 |

Continued on next page

TABLE S1 – continued from previous page

| **Chemical formula** | **Space group** | **DFT predictions** (eV) | | |
|---|---|---|---|---|
| | | $\varepsilon_g$ | $E_{VB}$ | $E_{CB}$ |
| $Cs_3BiO_3$ | $P2_13$ | 3.26 | 1.69 | –1.57 |
| $Cs_6Bi_4O_9$ | $P\bar{1}$ | — | — | — |
| $Sr(BiO_2)_2$ | $C2/m$ | — | — | — |
| $Sr_2Bi_2O_5$ | $Pnma$ | 2.23 | 2.43 | 0.20 |
| $Ba_2Bi_2O_5$ | $P2_1/c$ | 1.88 | 2.49 | 0.61 |

## II. PROJECTED DENSITY OF STATES BEFORE AND AFTER SELF-INTERACTION CORRECTION

After screening the 109 materials based on band edges and band gaps, the list of potential photocatalysts was reduced to 25 compounds. To proceed and select the orbitals on which to apply the Hubbard $U$ corrections, the atomic-orbital-projected density of states (PDOS) of these 25 compounds were computed. The PDOSs obtained within DFT and DFT+$U$ are represented in Fig. S1 and in Fig. S2, respectively. They show that O-2$p$ orbitals contribute the most to band-edges states; in particular, they dominate states near the top of the valence band, while states at the minimum of the conduction band are a mixture of O-2$p$ orbitals, and $s$ and $p$ states from the $p$-block element. Hence, Hubbard $U$ corrections were applied only to the O-2$p$ states.

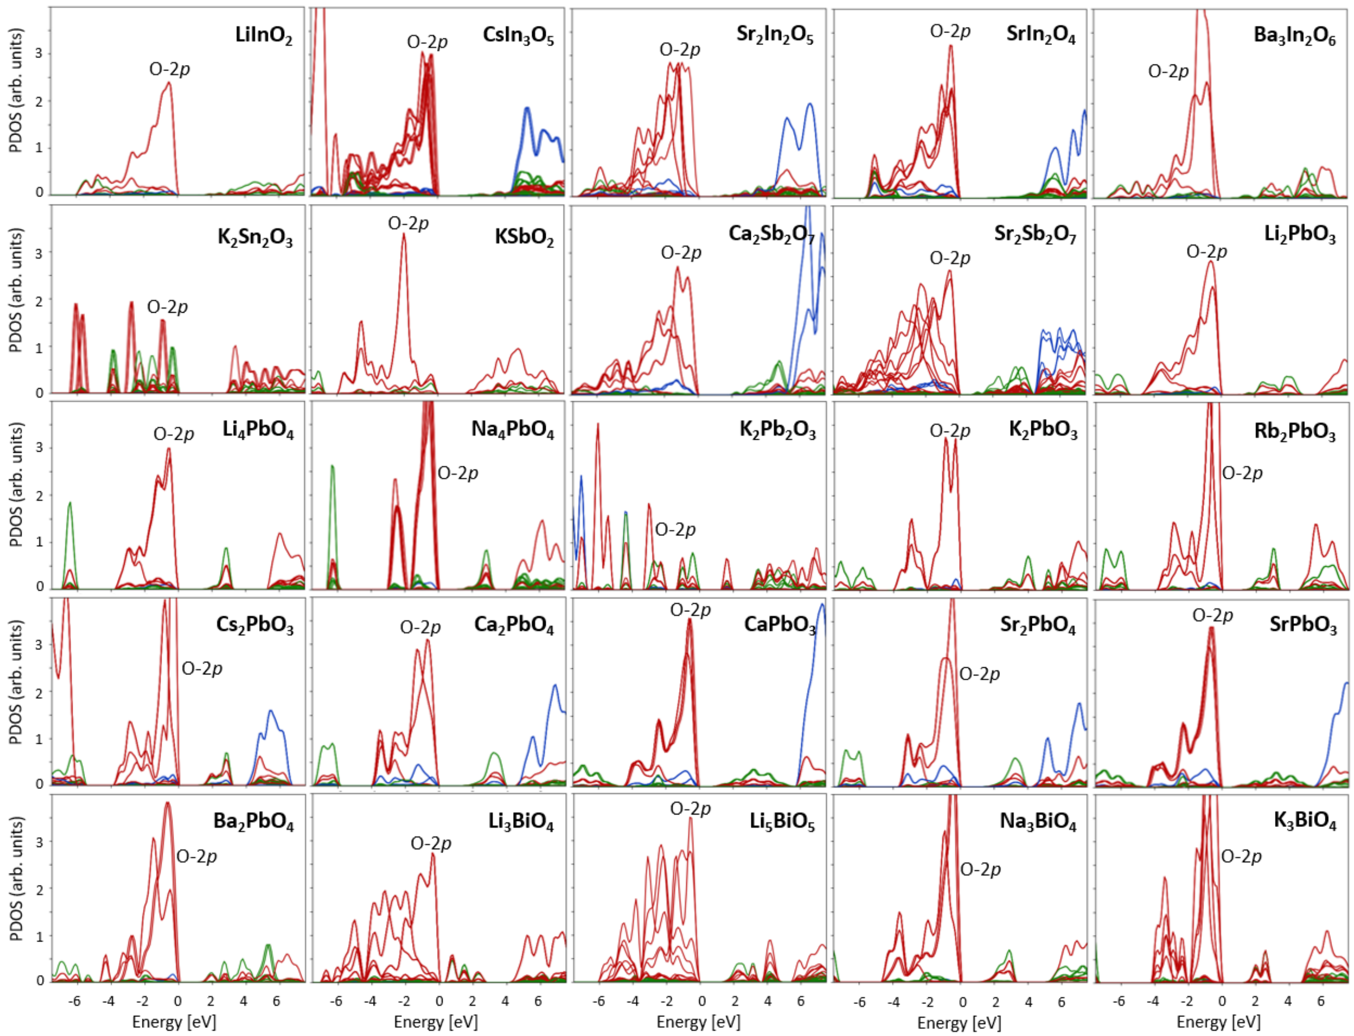


FIG. S1. Projected density of states (PDOS) from DFT for the 25 materials screened out by the band gap and band edge screening criteria. The plots are color-coordinated so that $s$ states are in green, $p$ states are in red, and $d$ states are in blue. The point of zero energy is referenced to the valence band maximum for all materials. Note that cases where there are multiple lines of the same color indicate symmetry non-equivalent atoms (e.g., multiple red lines for $Li_5BiO_5$ labeled as O-2$p$ are the 2$p$ states of non-equivalent oxygen atoms).

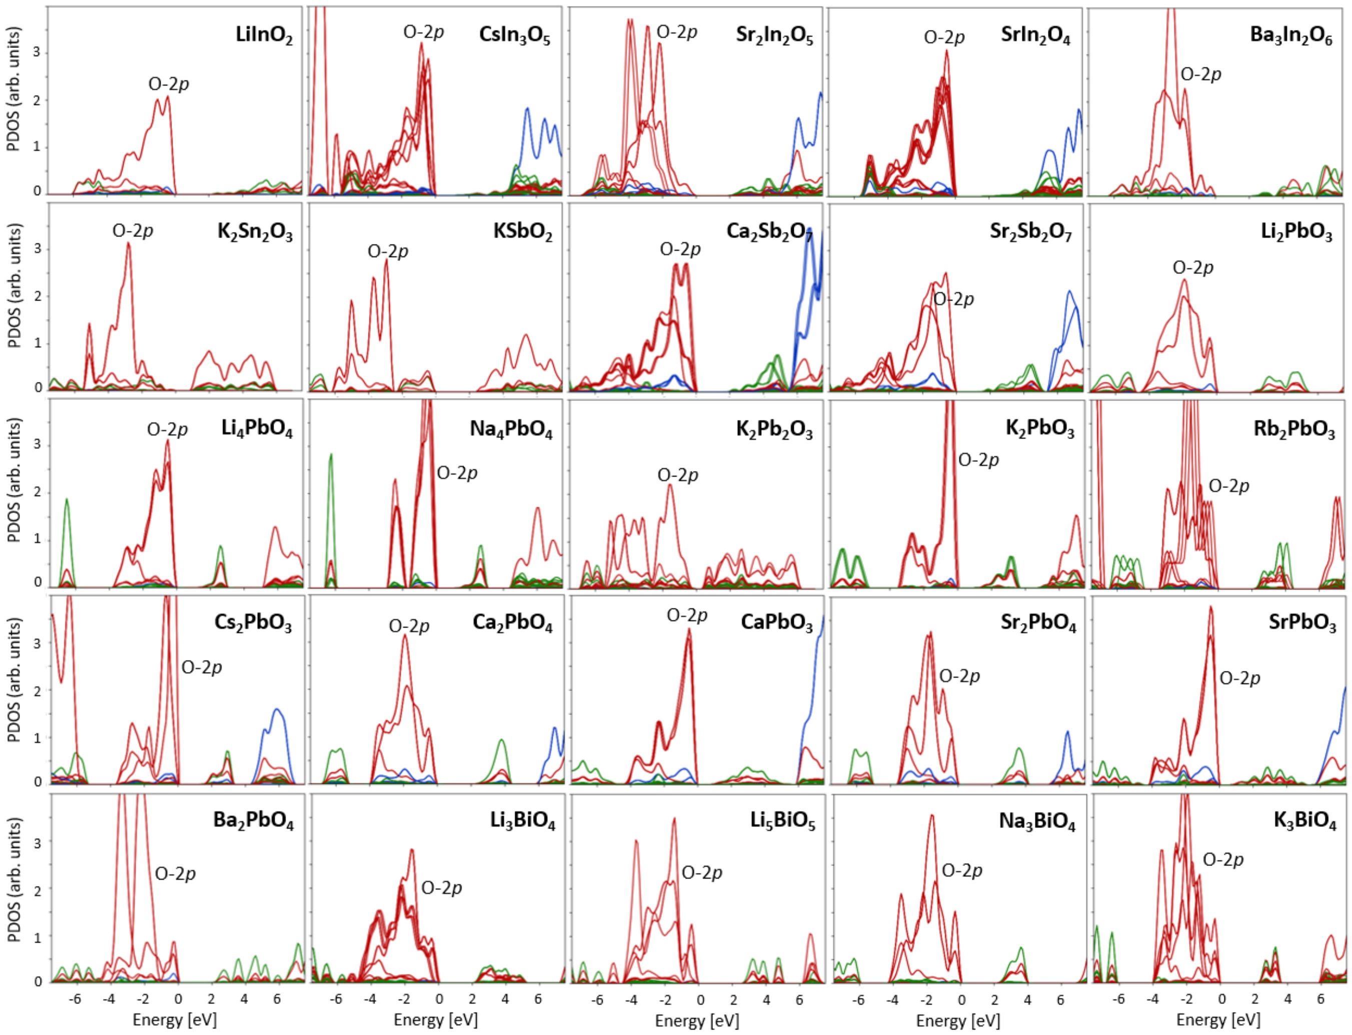


FIG. S2. Projected density of states (PDOS) from DFT+$U$ for the 25 materials screened out by the band gap and band edge screening criteria at the level of DFT. The plots are color-coordinated so that $s$ states are in green, $p$ states are in red, and $d$ states are in blue. The point of zero energy is referenced to the valence band maximum for all materials. Note that cases where there are multiple lines of the same color indicate symmetry non-equivalent atoms (e.g., multiple red lines for $Li_5BiO_5$ labeled as O-2$p$ are the 2$p$ states of non-equivalent oxygen atoms).

## III. ELECTROCHEMICAL STABILITY FROM COMPUTED POURBAIX DIAGRAMS

To assess their stability in water, the Pourbaix diagrams (Fig. S3) of the 19 compounds remaining at the last step of the screening protocol were evaluated at standard conditions of 298 K and 1 atm, and at an ionic concentration of $10^{-6}$ M, using the *pourbaix_diagram* module of the pymatgen (Python Materials Genomics) package [1–3]. The relative variations of Gibbs free energy with respect to the most stable phase were computed for each material, at their flatband potential and at pH 7 (Fig. S4). The resulting decomposition energies, together with the stable decomposition products, are reported in Table S2.

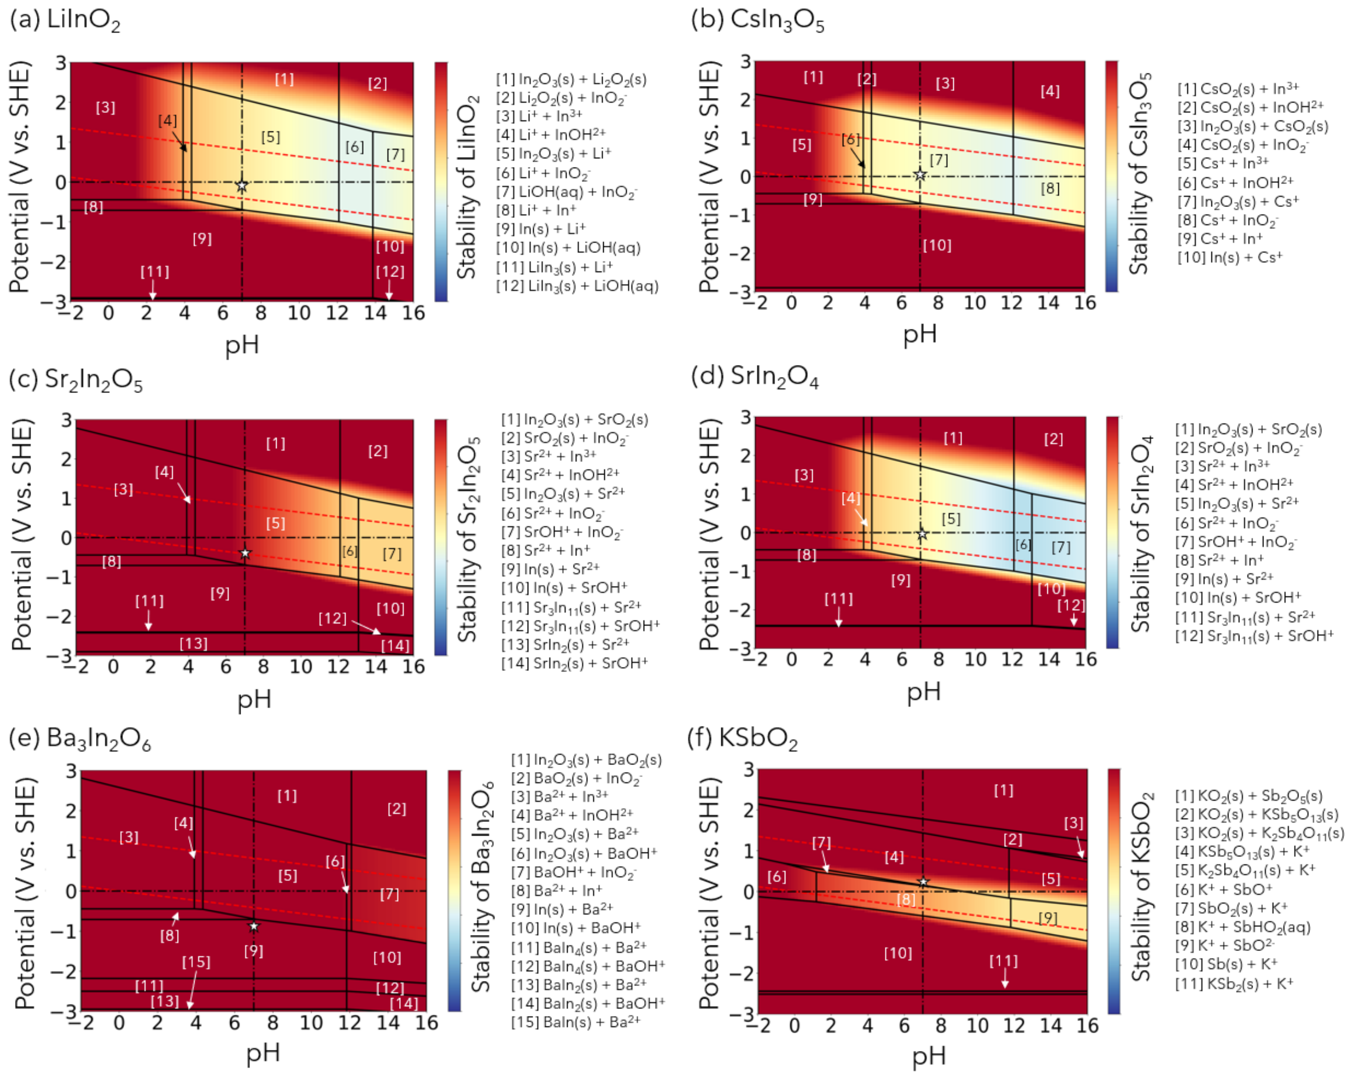

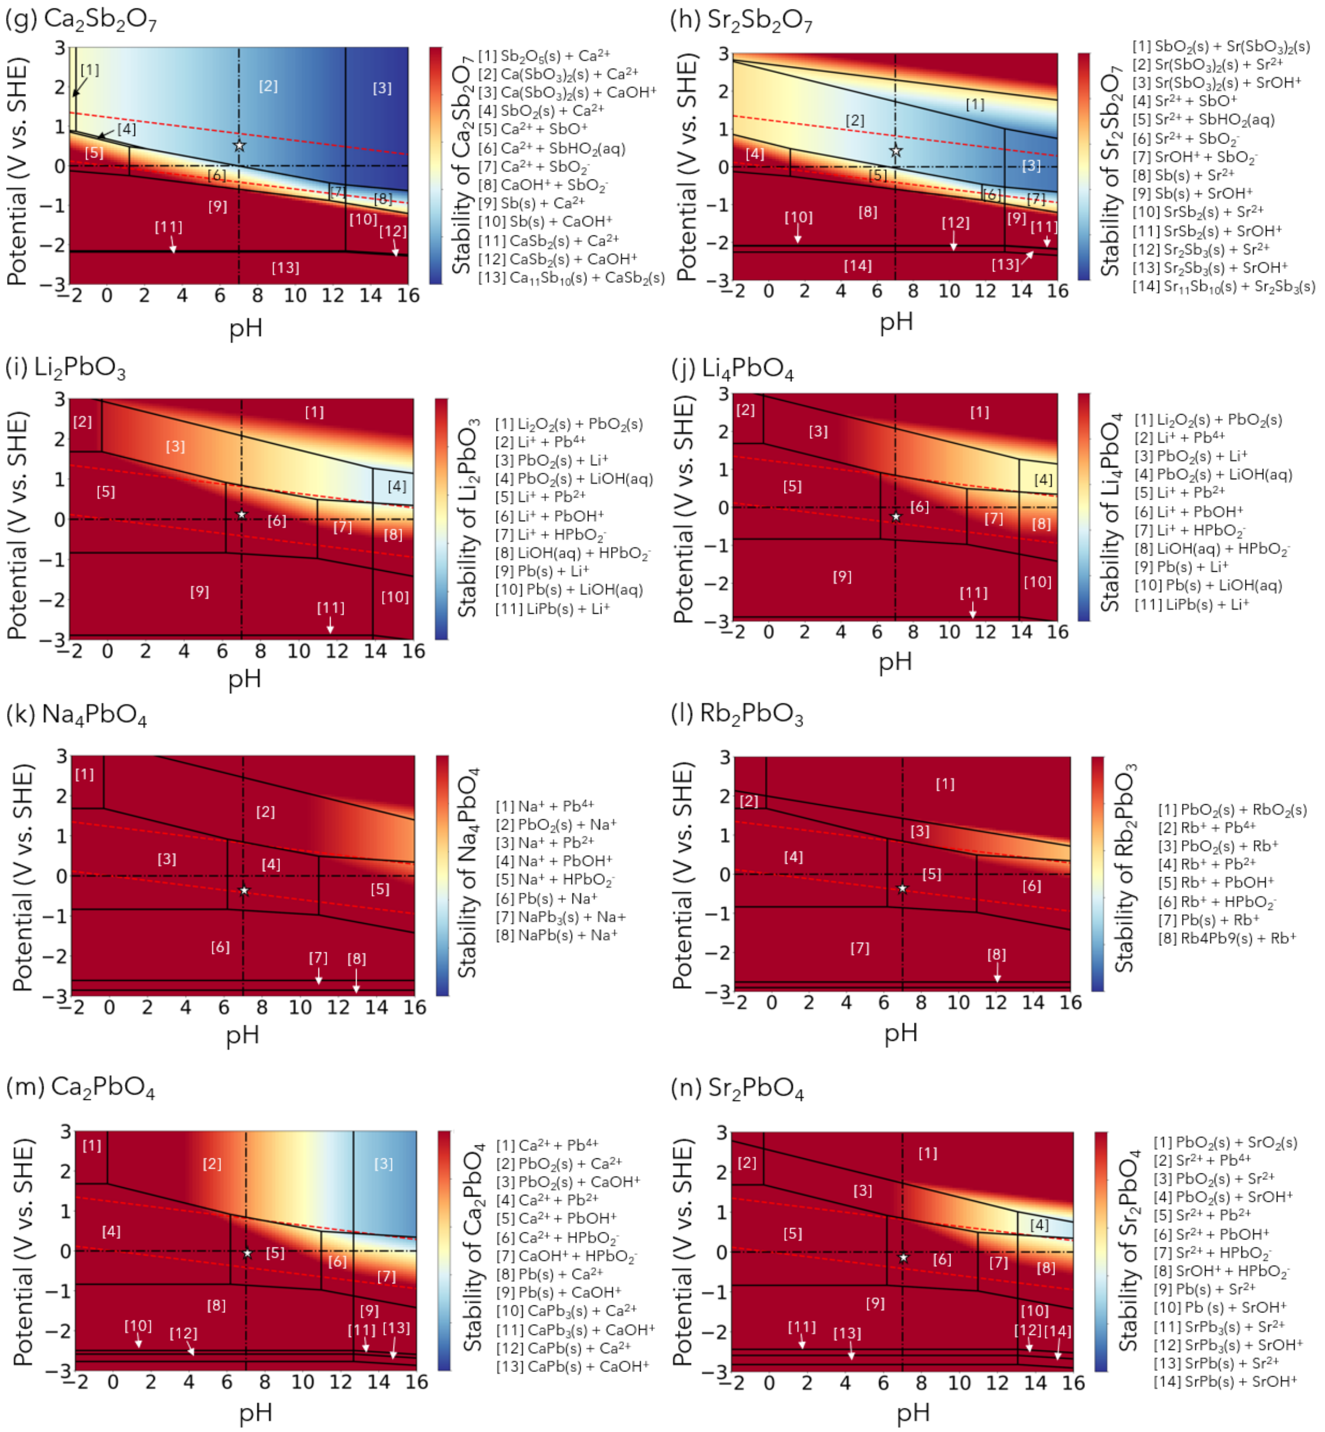

(g) Ca2Sb2O7
[1] Sb2O5(s) + Ca2+
[2] Ca(SbO3)2(s) + Ca2+
[3] Ca(SbO3)2(s) + CaOH+
[4] SbO2(s) + Ca2+
[5] Ca2+ + SbO+
[6] Ca2+ + SbHO2(aq)
[7] Ca2+ + SbO2-
[8] CaOH+ + SbO2-
[9] Sb(s) + Ca2+
[10] Sb(s) + CaOH+
[11] CaSb2(s) + Ca2+
[12] CaSb2(s) + CaOH+
[13] Ca11Sb10(s) + CaSb2(s)
Stability of Ca2Sb2O7
(h) Sr2Sb2O7
[1] SbO2(s) + Sr(SbO3)2(s)
[2] Sr(SbO3)2(s) + Sr2+
[3] Sr(SbO3)2(s) + SrOH+
[4] Sr2+ + SbO+
[5] Sr2+ + SbHO2(aq)
[6] Sr2+ + SbO2-
[7] SrOH+ + SbO2-
[8] Sb(s) + Sr2+
[9] Sb(s) + SrOH+
[10] SrSb2(s) + Sr2+
[11] SrSb2(s) + SrOH+
[12] Sr2Sb3(s) + Sr2+
[13] Sr2Sb3(s) + SrOH+
[14] Sr11Sb10(s) + Sr2Sb3(s)
Stability of Sr2Sb2O7
(i) Li2PbO3
[1] Li2O2(s) + PbO2(s)
[2] Li+ + Pb4+
[3] PbO2(s) + Li+
[4] PbO2(s) + LiOH(aq)
[5] Li+ + Pb2+
[6] Li+ + PbOH+
[7] Li+ + HPbO2-
[8] LiOH(aq) + HPbO2-
[9] Pb(s) + Li+
[10] Pb(s) + LiOH(aq)
[11] LiPb(s) + Li+
Stability of Li2PbO3
(j) Li4PbO4
[1] Li2O2(s) + PbO2(s)
[2] Li+ + Pb4+
[3] PbO2(s) + Li+
[4] PbO2(s) + LiOH(aq)
[5] Li+ + Pb2+
[6] Li+ + PbOH+
[7] Li+ + HPbO2-
[8] LiOH(aq) + HPbO2-
[9] Pb(s) + Li+
[10] Pb(s) + LiOH(aq)
[11] LiPb(s) + Li+
Stability of Li4PbO4
(k) Na4PbO4
[1] Na+ + Pb4+
[2] PbO2(s) + Na+
[3] Na+ + Pb2+
[4] Na+ + PbOH+
[5] Na+ + HPbO2-
[6] Pb(s) + Na+
[7] NaPb3(s) + Na+
[8] NaPb(s) + Na+
Stability of Na4PbO4
(l) Rb2PbO3
[1] PbO2(s) + RbO2(s)
[2] Rb+ + Pb4+
[3] PbO2(s) + Rb+
[4] Rb+ + Pb2+
[5] Rb+ + PbOH+
[6] Rb+ + HPbO2-
[7] Pb(s) + Rb+
[8] Rb4Pb9(s) + Rb+
Stability of Rb2PbO3
(m) Ca2PbO4
[1] Ca2+ + Pb4+
[2] PbO2(s) + Ca2+
[3] PbO2(s) + CaOH+
[4] Ca2+ + Pb2+
[5] Ca2+ + PbOH+
[6] Ca2+ + HPbO2-
[7] CaOH+ + HPbO2-
[8] Pb(s) + Ca2+
[9] Pb(s) + CaOH+
[10] CaPb3(s) + Ca2+
[11] CaPb3(s) + CaOH+
[12] CaPb(s) + Ca2+
[13] CaPb(s) + CaOH+
Stability of Ca2PbO4
(n) Sr2PbO4
[1] PbO2(s) + SrO2(s)
[2] Sr2+ + Pb4+
[3] PbO2(s) + Sr2+
[4] PbO2(s) + SrOH+
[5] Sr2+ + Pb2+
[6] Sr2+ + PbOH+
[7] Sr2+ + HPbO2-
[8] SrOH+ + HPbO2-
[9] Pb(s) + Sr2+
[10] Pb (s) + SrOH+
[11] SrPb3(s) + Sr2+
[12] SrPb3(s) + SrOH+
[13] SrPb(s) + Sr2+
[14] SrPb(s) + SrOH+
Stability of Sr2PbO4
Potential (V vs. SHE)
pH

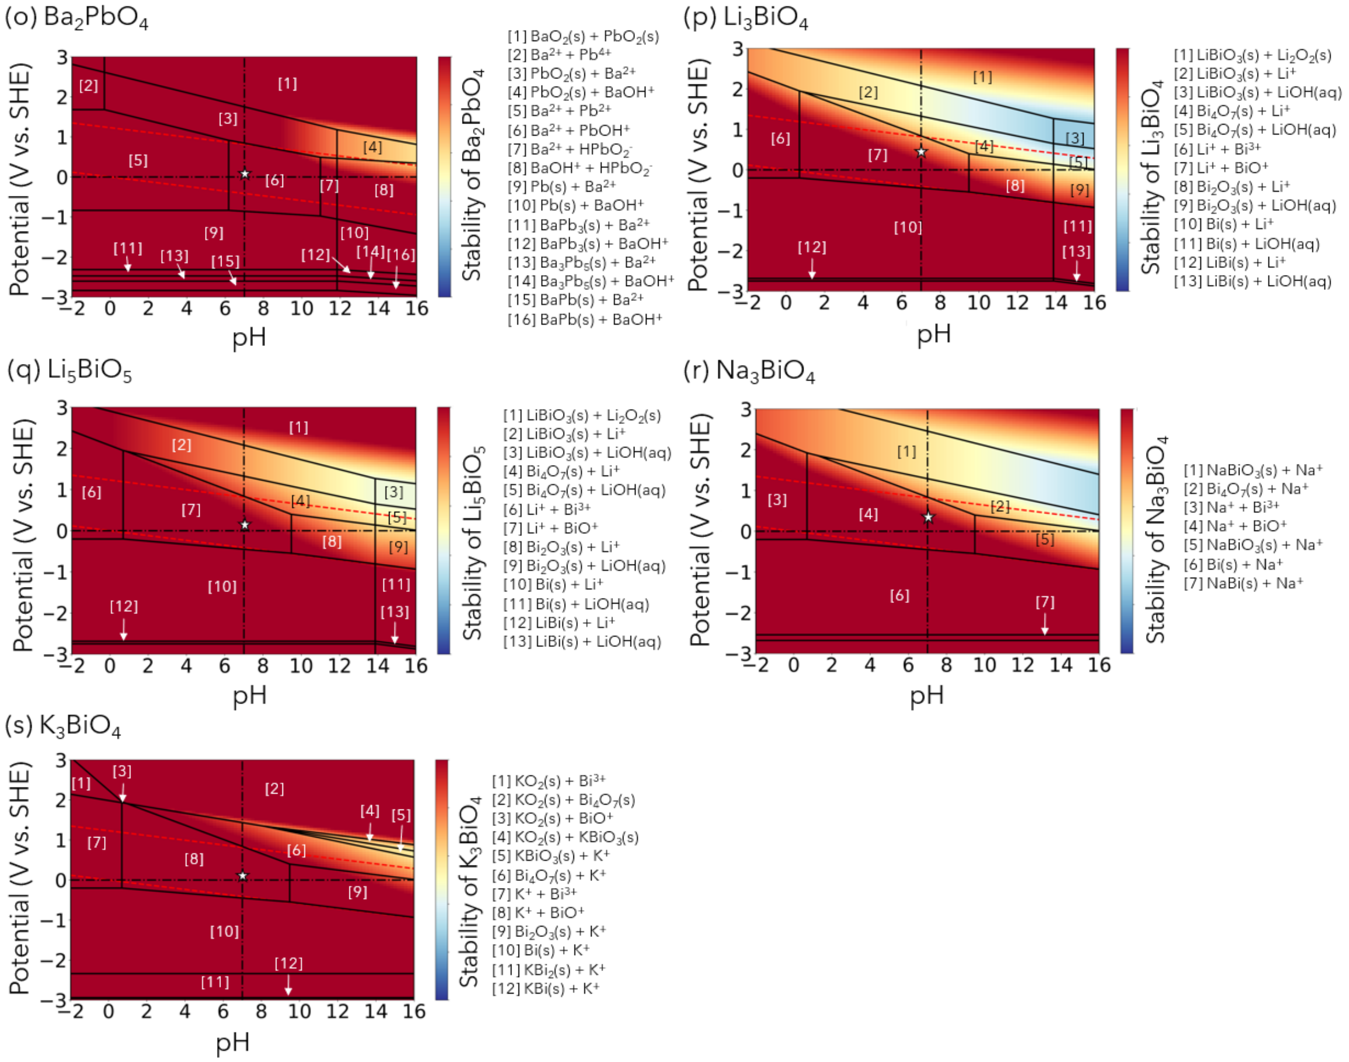


FIG. S3. Pourbaix diagrams for the 19 materials remaining after screening for band gap and band alignment at both the DFT and DFT+$U$ levels of theory. The colormap represents the difference in Gibbs free energy between the studied material and the Pourbaix stable phases: blue and red colors indicate regions of high and low stability, respectively. The white star on each diagram indicates the flatband potential of the given material at pH 7. The red dotted lines indicate the water redox potentials. The black dotted lines indicate pH 7 and potential of 0 V.

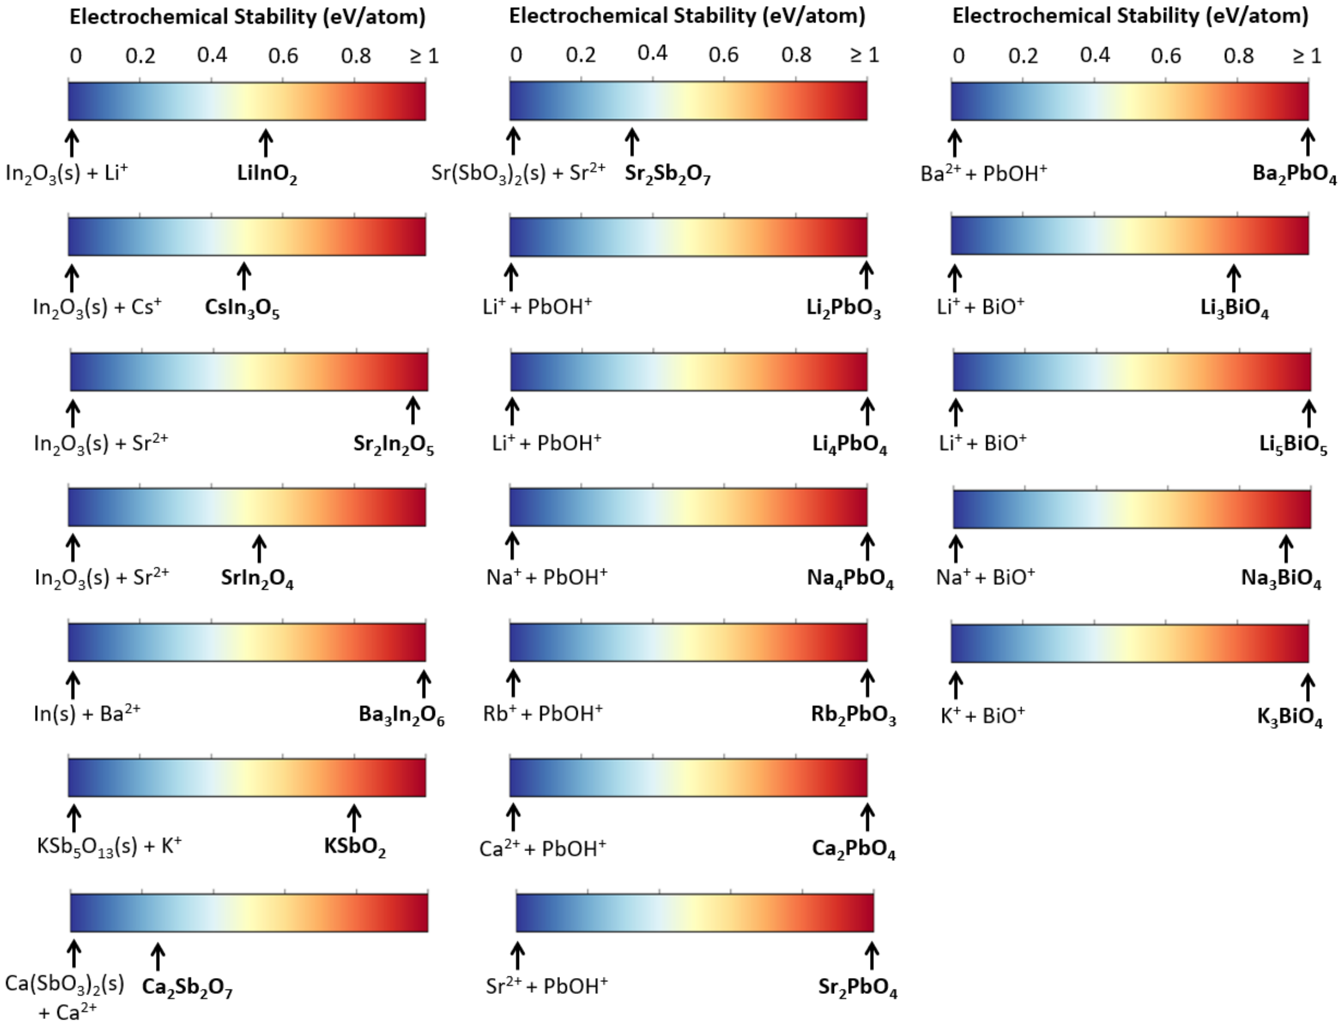


FIG. S4. Electrochemical stabilities and stable decomposition products for the 19 materials remaining after screening for band gap and band alignment at both the DFT and DFT+$U$ levels of theory. The electrochemical stability and stable decomposition products were measured at pH 7 and the flatband potential of the material.

TABLE S2. Pourbaix diagram data for the 19 ternary oxides of $s$- and $p$-block metal elements screened based on band gap and band edges. The seven compounds remaining after the water stability analysis are highlighted in bold. The band gap is given at the DFT+$U$ level of theory. The decomposition energy and stable decomposition products were extracted from the Pourbaix diagrams in Fig. S3 and are given for each material at their flatband potential and pH 7.

| **Chemical Formula** | **DFT+$U$** $\varepsilon_g$ (eV) | **Flatband potential** (eV) | **Decomposition energy** (eV/atom) | **Stable decomposition products** |
|---|---|---|---|---|
| **$LiInO_2$** | 3.94 | –0.05 | 0.57 | $In_2O_3$(s) + $Li^+$ |
| **$CsIn_3O_5$** | 3.42 | 0.03 | 0.49 | $In_2O_3$(s) + $Cs^+$ |
| **$Sr_2In_2O_5$** | 2.25 | –0.39 | 0.95 | $In_2O_3$(s) + $Sr^{2+}$ |
| **$SrIn_2O_4$** | 3.92 | –0.01 | 0.53 | $In_2O_3$(s) + $Sr^{2+}$ |
| $Ba_3In_2O_6$ | 2.66 | –0.82 | 1.46 | In(s) + $Ba^{2+}$ |
| **$KSbO_2$** | 2.82 | 0.23 | 0.80 | $KSb_5O_{13}$(s) + $K^+$ |
| **$Ca_2Sb_2O_7$** | 4.09 | 0.71 | 0.22 | $Ca(SbO_3)_2$(s) + $Ca^{2+}$ |
| **$Sr_2Sb_2O_7$** | 3.66 | 0.61 | 0.33 | $Sr(SbO_3)_2$(s) + $Sr^{2+}$ |
| $Li_2PbO_3$ | 2.08 | 0.12 | 1.14 | $Li^+$ + $PbOH^+$ |
| $Li_4PbO_4$ | 3.04 | –0.19 | 1.26 | $Li^+$ + $PbOH^+$ |
| $Na_4PbO_4$ | 3.22 | –0.31 | 1.61 | $Na^+$ + $PbOH^+$ |
| $Rb_2PbO_3$ | 2.45 | –0.28 | 1.76 | $Rb^+$ + $PbOH^+$ |
| $Ca_2PbO_4$ | 2.47 | –0.03 | 1.31 | $Ca^{2+}$ + $PbOH^+$ |
| $Sr_2PbO_4$ | 2.32 | –0.16 | 1.61 | $Sr^{2+}$ + $PbOH^+$ |
| $Ba_2PbO_4$ | 2.36 | 0.10 | 1.64 | $Ba^{2+}$ + $PbOH^+$ |
| $Li_3BiO_4$ | 2.41 | 0.57 | 0.80 | $Li^+$ + $BiO^+$ |
| $Li_5BiO_5$ | 2.82 | 0.16 | 1.07 | $Li^+$ + $BiO^+$ |
| $Na_3BiO_4$ | 2.42 | 0.46 | 0.93 | $Na^+$ + $BiO^+$ |
| $K_3BiO_4$ | 2.60 | 0.14 | 1.41 | $K^+$ + $BiO^+$ |

## IV. EXPERIMENTAL DATA FROM STRUCTURAL AND OPTICAL MEASUREMENTS

Out of the 109 initial candidate photocatalysts, seven were selected by the screening protocol described in the main text. To confirm the validity of this computational screening, four compounds ($LiInO_2$, $SrInO_4$, $Ca_2Sb_2O_7$, and $Sr_2Sb_2O_7$) were synthesized and characterized: by X-ray diffraction to assess phase stability (Fig. S5), by Tauc analysis to evaluate band gaps (Fig. S6), and by chopped-illumination voltammetry to determine the flatband potential (Fig. 4b, main text).

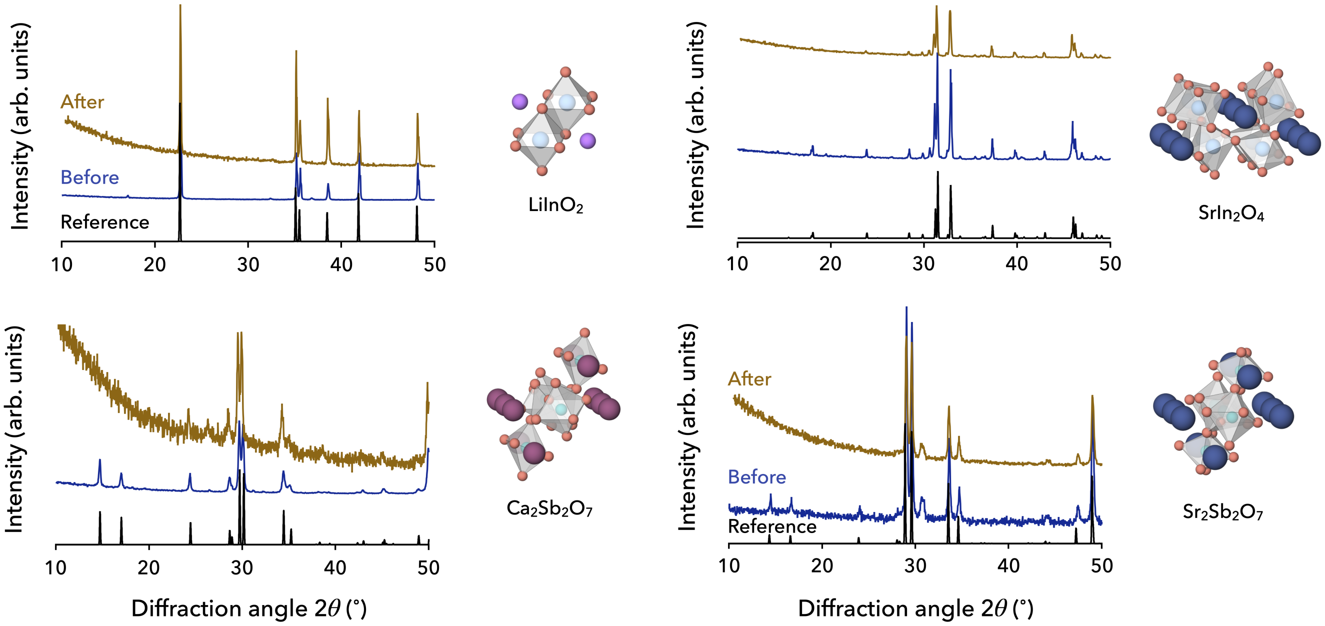


FIG. S5. X-ray diffraction of the four compounds synthesized in this study. From bottom to top, X-ray signals correspond to reference patterns (black lines), diffraction of samples before photocatalysis (blue lines), and after photocatalysis (brown lines). The photocatalysis step induces only little variations of X-ray diffraction, suggesting that compounds are stable in water.

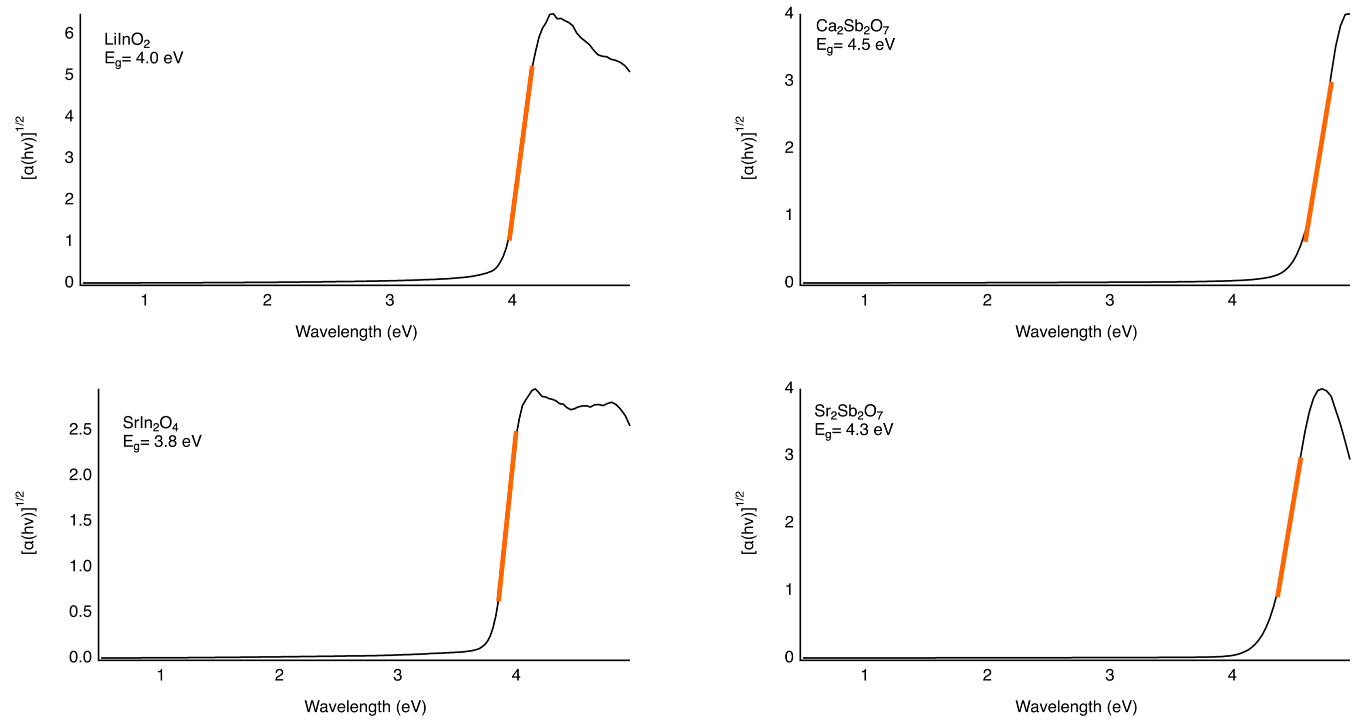


FIG. S6. Tauc plots of the four compounds analyzed in Fig. S5. Band gaps are evaluated by linear extrapolation of the Tauc signal.


[1] S. P. Ong, W. D. Richards, A. Jain, G. Hautier, M. Kocher, S. Cholia, D. Gunter, V. L. Chevrier, K. A. Persson, and G. Ceder, Python materials genomics (pymatgen): A robust, open-source python library for materials analysis, Computational Materials Science **68**, 314 (2013).

[2] K. A. Persson, B. Waldwick, P. Lazic, and G. Ceder, Prediction of solid-aqueous equilibria: Scheme to combine first-principles calculations of solids with experimental aqueous states, Physical Review B **85**, 235438 (2012).

[3] A. K. Singh, L. Zhou, A. Shinde, S. K. Suram, J. H. Montoya, D. Winston, J. M. Gregoire, and K. A. Persson, Electrochemical stability of metastable materials, Chemistry of Materials **29**, 10159 (2017).
